# Supplementary material for: Is It Worth the Attention? A Comparative Evaluation of Attention Layers for Argument Unit Segmentation
Source: arXiv:1906.10068 source file (2019-06-24)
Supplement: Supplementary file 1 [file 08-appendix.tex]

\section{Appendices}
\label{sec:appendix}
TODO
